# Supplementary material for: FastCap: An Efficient and Fair Algorithm for Power Capping in Many-Core Systems
Source: arXiv:1603.01313 source file (2016-03-03)
Supplement: Supplementary file 1 [file appendix.tex]

\section*{Appendix}

\noindent{\bf Proof of Theorem~\ref{thm.equality}.}
We first show that constraint \eqref{eq.powerConstraint} must be equality. Suppose otherwise, then we can always reduce the optimal bus speed $s_b^*$ such that the performance of each core is improved (because of the decrease in $R$). As the result we can achieve a better objective which is larger than $D^*$. This leads to a contradiction. Thus the power budget constraint must be equality. 

Then we show that constraint \eqref{eq.perfConstraint} must also be equality. Suppose otherwise, i.e., there exists a $j$ such that \eqref{eq.perfConstraint} is strictly smaller than $D^* T_j$. Then we can always increase the $z_j^*$. The power budget saved from this core can be redistributed to other cores that have equalities in \eqref{eq.perfConstraint}. As the result we can achieve a better objective which is larger than $D^*$. This leads to a contradiction.
